# Supplementary material for: Unraveling Misinformation Propagation in LLM Reasoning
Source: arXiv:2505.18555 source file (2025-09-23)
Supplement: Supplementary file 1 [file soc.tex]

\section{Overview of Changes}

We have expanded our previous short paper to a long one. Below covers the significant changes in our new paper.

\subsection{Reorganization of Claims and Contributions}

\begin{itemize}
    \item \textbf{\Section~\ref{sec:main:robustness:default} (Tendency to Follow Misinformation):} We now emphasize that models, by default, treat misinformation as part of the instruction. Therefore, performance decline and misinformation-following behavior in this setting are an expected baseline, not necessarily a "vulnerability" in itself. This section establishes \textit{why} explicit instructions are needed if correction is the desired outcome.
    \item \textbf{\Section~\ref{sec:main:correction_methods:prompting} (Instruct to Correct Misinformation):} We dedicate this section to experiments where models are explicitly instructed to correct misinformation. The findings that models still struggle to correct misinformation with explicit instructions demonstrate their vulnerability and limited steerability even under direct guidance.
    \item \textbf{\Section~\ref{sec:main:controlled} (Mitigating Propagation via Correction):} This new section explores the effectiveness of early factual corrections and fine-tuning as strategies to mitigate the propagation of misinformation.
\end{itemize}

\subsection{Comprehensive Comparison With Related Work}

\begin{itemize}
    \item Moved the Related Work section from the appendix to \Section~\ref{sec:main:related}.
    \item Organization and Wording: split ``User Misinformation Propagation'' into two sub-domains: ``Misinformation in LLM Interaction'' and ``Error Propagation''; renamed ``Handling Conflicts Between User and Model'' to ``User-Model Knowledge Conflicts''.
    \item Included more literature for comparison; elaborated on how related work is limited and our work is different from them (paragraph 2 in \Section~\ref{fig:intro}, \Section~\ref{sec:main:related}).
\end{itemize}

\subsection{Additional Experiments}

\begin{itemize}
    \item Conducted additional experiments which explicitly instruct models to follow misinformation: covered part of them in \Section~\ref{sec:main:robustness:default} and \Table~\ref{tab:main_results}; added a new section \Appendix~\ref{sec:appendix:inst_follow}.
    \item Added the evaluation of misinformation-following behavior from the appendix to the main body: added \Figure~\ref{fig:sankey_perturbed}; influenced \Section~\ref{sec:main:setup:evaluation}.
    \item Updated analysis of the relation between relative performance decrease and difficulty gradation: changed the experiment setting that explicitly instructs LLMs to correct misinformation; moved analysis of Pearson correlation from the appendix to the main body (\Figure~\ref{fig:bar}).
    \item Added fine-tuning experiments for misinformation mitigation from the appendix to \Section~\ref{sec:main:controlled:finetuning}; influenced \Figure~\ref{fig:sankey_ft} and \Table~\ref{tab:finetune}.
\end{itemize}

\subsection{Change of Wordings}

\begin{itemize}
    \item Changed ``Error Propagation from User Misinformation'' to ``Misinformation Propagation'' since it is not appropriate to treat misinformation as errors, as reviewers suggest. And we focus on how LLMs handle misinformation in various forms of input, not limited to a specific source, e.g., user. 
    \item Split the original ``Analysis Framework'' subsection in \Section~\ref{sec:main:setup} into ``Experiment Design'' (\Section~\ref{sec:main:setup:analysis}) and ``Evaluation Framework'' (\Section~\ref{sec:main:setup:evaluation}).
    \item Replaced the ``\textcolor{customgreen}{prompting} setting'' with the ``\textcolor{customgreen}{\prompting} instruction'' (explicitly asking LLMs to correct misinformation) and the ``\textcolor{customgreen}{\following} instruction'' (explicitly asking LLMs to follow misinformation).
\end{itemize}

\subsection{Figures and Tables}

\begin{itemize}
    \item \Figure~\ref{fig:intro}: Added explicit instructions to correct misinformation; changed the wording to ``misinformation propagation''.
    \item \Figure~\ref{fig:pipeline}: Added this overall pipeline figure for better understanding.
    \item \Table~\ref{tab:main_results}: Added results of explicit instructions to follow misinformation; added relative decrease and 95\% confidence interval.
    \item \Figure~\ref{fig:sankey_perturbed}: Added this to evaluate whether models follow misinformation in their reasoning steps.
    \item \Figure~\ref{fig:bar}: Adjusted it to a double-column figure; added results of Pearson correlation between relative performance decrease and question difficulty gradation.
    \item \Figure~\ref{fig:pathway}: Adjusted it to a double-column figure.
    \item \Figure~\ref{fig:sankey_ft} and \Table~\ref{tab:finetune}: Added them for the new fine-tuning experiments.
\end{itemize}

\section{Point-By-Point Response to Each Weakness and Suggestion}

\subsection{Meta Reviewer PAgJ}

\begin{itemize}
    \item Several reviewers question whether it is appropriate to treat models following user misinformation as being ``misled.'' Since instruction-following is a core behavior of LLMs, blindly labeling this behavior as erroneous may be problematic without clearer framing. \textcolor{blue}{Revision:
    (\textit{i}) We have conducted an additional experiment in \Section~\ref{sec:main:robustness:default} and \Appendix~\ref{sec:appendix:inst_follow} and emphasized that models, by default, treat misinformation as user instruction and follow it. Thus, models require explicit correction instructions to rectify misinformation (lines 354-363).
    (\textit{ii}) Our evaluation of correction capability is primarily focused on scenarios where models are explicitly instructed to correct misinformation (lines 014-017, 043-049, 095-099, and \Section~\ref{sec:main:correction_methods:prompting}).}
    \item The paper does not adequately compare its findings with prior work on error propagation in CoT reasoning, missing an opportunity to differentiate its contributions. \textcolor{blue}{Revision:
    (\textit{i}) We have differentiated misinformation as part of instructions from model internal errors in both distribution and effects on model reasoning (lines 062-071).
    (\textit{ii}) We have also comprehensively compared our work with all related work in \Section~\ref{sec:main:related}.}
    \item Some reviewers raise concerns that the setting may be overly artificial or constructed. The motivation for studying this as a real-world problem could be better justified. \textcolor{blue}{Revision:
    (\textit{i}) We have emphasized that misinformation is a prevalent issue in real-world LLM interactions (lines 037-059).
    (\textit{ii}) Our misinformation is designed based on common human error patterns to reflect realistic scenarios (lines 079-085).}
\end{itemize}

\subsection{Reviewer MJ6j}

\begin{itemize}
    \item Models are not expected to correct user misinformation by their default instruction-following design. Their misinformation-following behaviors are not erroneous. \textcolor{blue}{Revision:
    (\textit{i}) We have conducted an additional experiment in \Section~\ref{sec:main:robustness:default} and \Appendix~\ref{sec:appendix:inst_follow} and emphasized that models, by default, treat misinformation as user instruction and follow it. Thus, models require explicit correction instructions to rectify misinformation (lines 354-363).
    (\textit{ii}) Our evaluation of correction capability is primarily focused on scenarios where models are explicitly instructed to correct misinformation (lines 014-017, 043-049, 095-099, and \Section~\ref{sec:main:correction_methods:prompting}).}
    \item Definition of evaluation metric (K-Acc) is unclear. \textcolor{blue}{Revision: We have revised the explanation of \accuracy to interpret the meaning of original and misinformed \accuracy and to clarify why \accuracy is used over standard accuracy (lines 280-298).}
    \item Interpretation of Table 1 is complicated by original scores below 100\%, potentially affecting conclusions about misinformation impact. \textcolor{blue}{Revision: We have explicitly added and discuss relative performance declines in Table~\ref{tab:main_results}.}
    \item Figure 2 analysis should focus on relative performance decline from ‘Original’ rather than absolute values. \textcolor{blue}{Revision:
    (\textit{i}) We have emphasized the comparison of misinformed \accuracy with the original \accuracy (relative decline) rather than absolute values (lines 386-388).
    (\textit{ii}) We have added Pearson correlation analysis between the relative performance decline and question difficulty (lines 391-395 and \Figure~\ref{fig:bar}).
    (\textit{iii}) To avoid confusion, we have removed phrases like "consistent performance drop" and "irrelevant to question difficulty." Instead, we now state that performance decreases across all models and difficulty levels, and report that no significant correlation was found between the relative performance decrease and the difficulty level based on our analysis.}
    \item Correction position analysis may unsurprisingly reflect larger models' superior instruction-following capabilities. \textcolor{blue}{Revision: We have revised the takeaways for this analysis to emphasize the importance of early and factual corrections for all models, rather than focusing on trends across model sizes (line 423).}
    \item Some of the writing (Figure 4 caption) could be improved. \textcolor{blue}{Revision: We have reviewed and revised captions and other text for clarity, including the caption for the relevant figure (now \Figure~\ref{fig:pathway}).}
\end{itemize}

\subsection{Reviewer A7Ud}

\begin{itemize}
    \item Models are not expected to correct user misinformation by their default instruction-following design. \textcolor{blue}{Revision:
    (\textit{i}) We have conducted an additional experiment in \Section~\ref{sec:main:robustness:default} and \Appendix~\ref{sec:appendix:inst_follow} and emphasized that models, by default, treat misinformation as user instruction and follow it. Thus, models require explicit correction instructions to rectify misinformation (lines 354-363).
    (\textit{ii}) Our evaluation of correction capability is primarily focused on scenarios where models are explicitly instructed to correct misinformation (lines 014-017, 043-049, 095-099, and \Section~\ref{sec:main:correction_methods:prompting}).}
    \item The research motivation seems artificial because the user misinformation collected is intentional or easily correctable. \textcolor{blue}{Revision:
    (\textit{i}) We have emphasized that misinformation is a prevalent issue in real-world LLM interactions (lines 037-059).
    (\textit{ii}) Our misinformation is designed based on common human error patterns to reflect realistic scenarios (lines 079-085).}
\end{itemize}

\subsection{Reviewer 6Dav}

\begin{itemize}
    \item Lack of comparison with previous works on error propagation. \textcolor{blue}{Revision:
    (\textit{i}) We have differentiated misinformation as part of instructions from model internal errors in both distribution and effects on model reasoning (lines 062-071).
    (\textit{ii}) We have also comprehensively compared our work with all related work in \Section~\ref{sec:main:related}.}
    \item The analysis in Figure 2 (Lines 188-193) lacks clear insight. \textcolor{blue}{Revision:
    (\textit{i}) We have emphasized the comparison of misinformed \accuracy with the original \accuracy (relative decline) rather than absolute values (lines 386-388).
    (\textit{ii}) We have added Pearson correlation analysis between the relative performance decline and question difficulty (lines 391-395 and \Figure~\ref{fig:bar}).
    (\textit{iii}) To avoid confusion, we have removed phrases like "consistent performance drop" and "irrelevant to question difficulty." Instead, we now state that performance decreases across all models and difficulty levels, and report that no significant correlation was found between the relative performance decrease and the difficulty level based on our analysis.}
    \item The meaning of using K-Accuracy as per-question accuracy is not clearly explained. \textcolor{blue}{Revision: We have revised the explanation of \accuracy to interpret the meaning of original and misinformed \accuracy and to clarify why \accuracy is used over standard accuracy (lines 280-298).
    (\textit{ii}) To prevent confusion, we have removed the term ``per-question accuracy'' from the \accuracy definition. The concept (used for difficulty gradation) is now explained separately in the context of \Figure~\ref{fig:bar} (lines 386-388, footnotes 9).}
\end{itemize}
